# Supplementary material for: eTOP: Early Termination of Pipelines for Faster Training of AutoML Systems
Source: arXiv:2304.08597 source file (2023-04-17)
Supplement: Supplementary file 2 [file appendix.notation.tex]

\subsection{Notation}\label{sec:appendic:notation}
