# Supplementary material for: eTOP: Early Termination of Pipelines for Faster Training of AutoML Systems
Source: arXiv:2304.08597 source file (2023-04-17)
Supplement: Supplementary file 3 [file appendix.tex]

\section{Appendix} \label{sec:appendix}
Extra detailed results here.
Negative Results. Genetic Algorithm.

\from{HZ}{Add details experiment setup for TPOT and AutoSklearn}
\from{HZ}{Add up to the notation table of new totations; and align the notations inside the paper}
\from{HZ}{Also add working example of what History H looks like in the appendix}

\subsection{Notation}\label{sec:appendic:notation}

\subsection{Algorithm}\label{sec:appendix:algorithm}
